# Supplementary material for: Real-time Visualization of Stream-based Monitoring Data
Source: arXiv:2205.12823 source file (2022-05-25)
Supplement: Supplementary file 1 [file appendix.tex]

\section{Appendix}\label{sec:appendix}

\begin{figure}[]
    \begin{minipage}{\linewidth}
        \centering
        \includegraphics[width=0.5\textwidth]{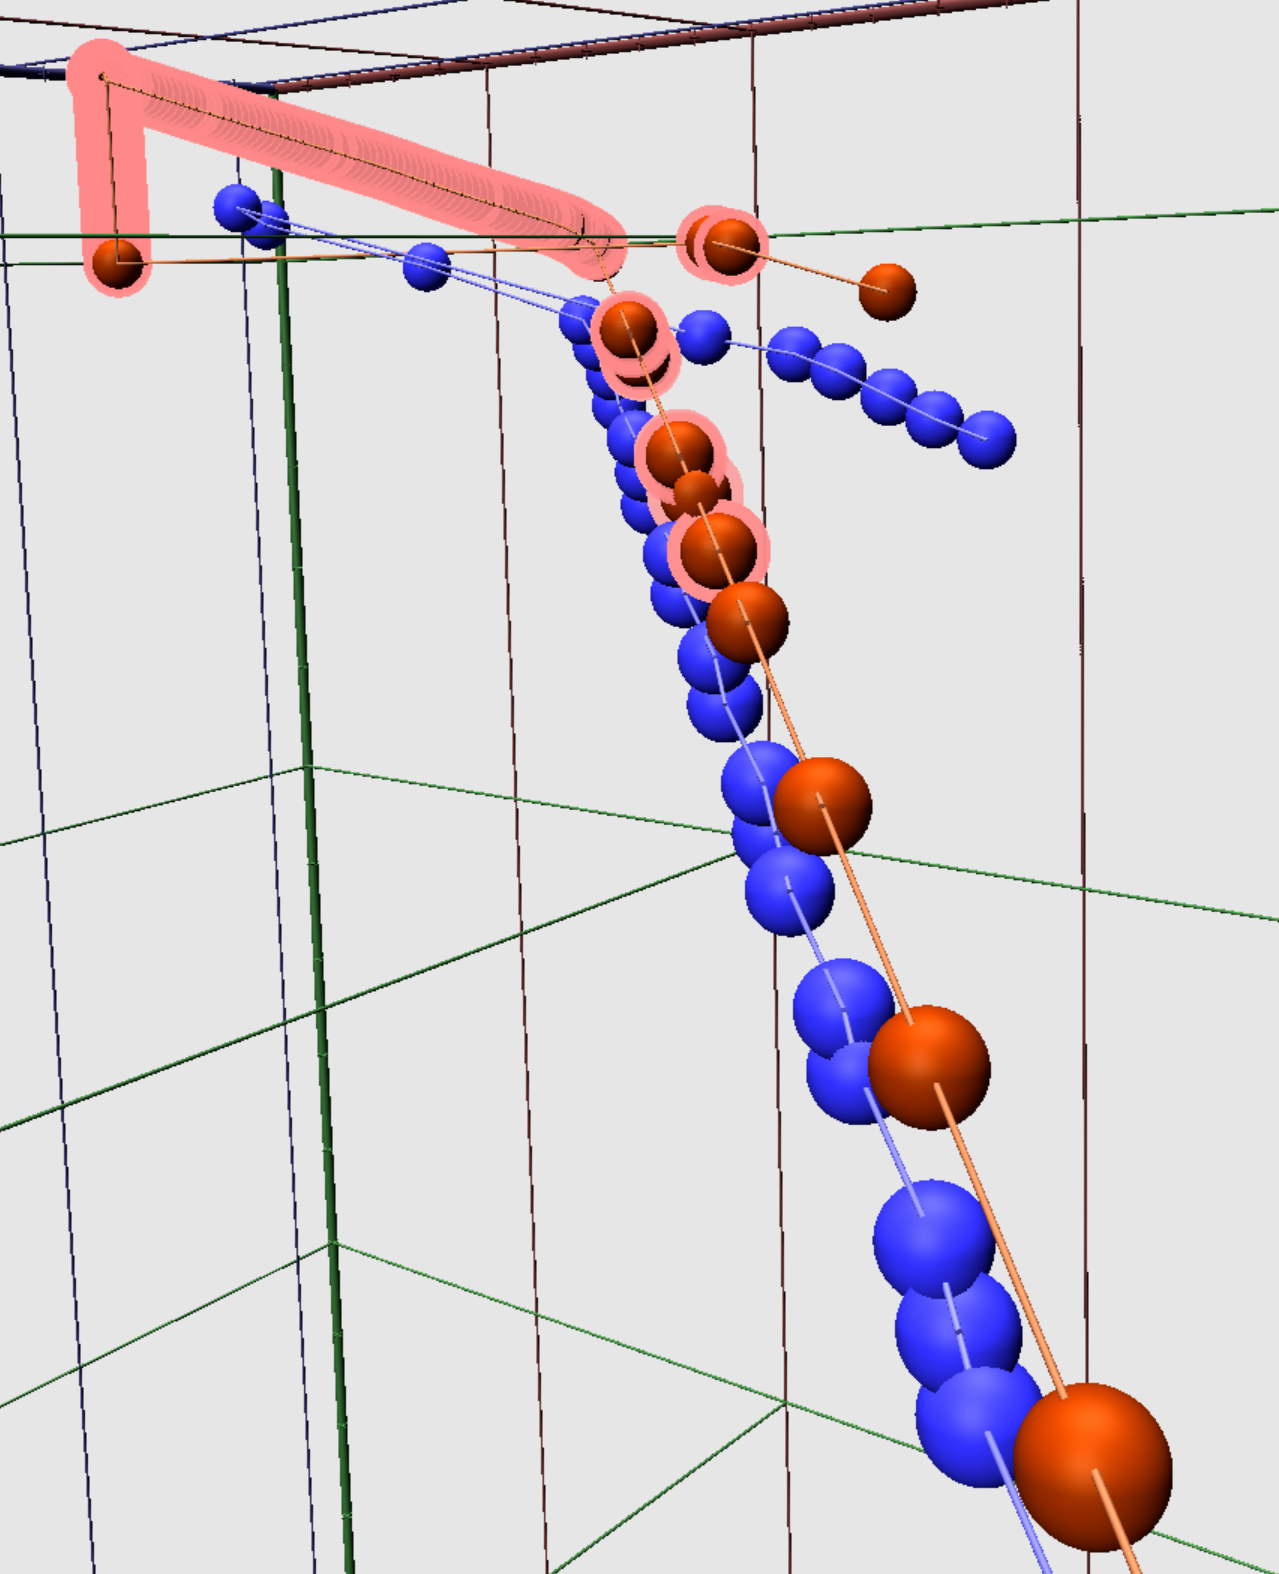}
    \end{minipage}
    \caption{The blue balls represent raw GPS positions and the orange balls represent estimated position after sensor fusion. A temporary failure of the GPS module was simulated, resulting in a change of visualization: every position estimate is plotted instead of plotting only after some distance and also a halo indicates the missing of GPS reading.}
    \label{fig:3d}
\end{figure}

% \todo{add comments from 3.2}
% \begin{figure}[t]
%     \input{specification32}
%     \caption{TODO}
%     \label{fig:specification32}
% \end{figure}
